# Supplementary material for: Computing Maxmin Strategies in Extensive-Form Zero-Sum Games with Imperfect Recall
Source: arXiv:1608.01510 source file (2017-05-24)
Supplement: Supplementary file 1 [file appendix.tex]

\section*{APPENDIX}

\section{LP for Strategy Reconstruction}
We provide a linear program that serves as a heuristic to compute a behavioral strategy in $I_1$, taking into account the realization probabilities $r(\sigma^k_1)$ of sequences $\sigma_1^k \in \seq{1}{I_1}$ leading to $I_1$ as well as errors that can be accumulated in the subtrees of individual histories $h \in I_1$ ($b^k$ is the behavioral strategy obtained for sequence $\sigma_1^k$, $b$ is the corrected one):

\vspace{-0.3cm}
{\small
\begin{subequations}\label{eq:strat_LP}
\begin{align}
\min_{b, L} & \sum_{\sigma_1^k \in \mathsf{seq}(I_1)} r(\sigma_1^k) \cdot L(\sigma_1^k)&&\label{eq:strat_LP:obj} \\
\text{s.t.} \qquad  L(\sigma_1^k) & = \sum_{a \in \calA(I_1)} L(\sigma_1^k,a) &&\forall \sigma_1^k \in \seq{1}{I_1}\label{eq:strat_LP:L_sum}\\
                  L(\sigma_1^k,a) & \geq [ b^k(a) - b(a) ] \cdot v_{max}(\sigma_1^k \cdot a)&&\forall \sigma_1^k \in \seq{1}{I_1}, \forall a \in \calA(I_1)\label{eq:strat_LP:L1} \\
                  L(\sigma_1^k,a) & \geq [ b(a) - b^k(a) ] \cdot (-v_{min}(\sigma_1^k \cdot a))&& \forall \sigma_1^k \in \seq{1}{I_1}, \forall a \in \calA(I_1)\label{eq:strat_LP:L2} \\
                  b(a) & = \sum_{\sigma_1^k \in \seq{1}{I_1}} \alpha(\sigma_1^k) \cdot b^k(a) && \forall a \in \calA(I_1) \label{eq:strat_LP:cvx1}\\
                  b(a) &\geq  b^k(a) &&\forall \sigma_1^k \in \seq{1}{I_1}\\
                  b(a) &\leq  b^k(a) &&\forall \sigma_1^k \in \seq{1}{I_1}\\
                  0 \leq \alpha(\sigma_1^k) & \leq 1 && \forall \sigma_1^k \in \seq{1}{I_1} \label{eq:strat_LP:cvx2}\\
                  \sum_{\sigma_1^k \in \seq{1}{I_1}} \alpha(\sigma_1^k) & = 1 &&\label{eq:strat_LP:cvx3}
            %      L(\sigma_1^k) & \in \mathbb{R} && \forall \sigma_1^k \in \mathsf{seq}(I_1) \\
              %    L(\sigma_1^k,a) & \in \mathbb{R} && \forall \sigma_1^k \in \mathsf{seq}(I_1) \forall a \in \calA(I_1)\label{eq:strat_LP:last}
\end{align}
\end{subequations}}

The LP finds the strategy minimizing the estimated error in the following way. Constraints \eqref{eq:strat_LP:L1},  \eqref{eq:strat_LP:L2} compute the maximum cost of changing the probability that action $a$ is played after $\sigma_1^k$ $ L(\sigma_1^k,a)$, assuming that the worst possible outcome in the subtree following playing $\sigma_1^ka$ is reached. Constraint \eqref{eq:strat_LP:L_sum} computes the estimated errors for every $\sigma_1^k$ $L(\sigma_1^k)$ by summing all the $L(\sigma_1^k, a)$ for all relevant $a$, and we minimize the sum of $L(\sigma_1^k)$ weighted by the realization probability of corresponding sequences in the objective. Constraints \eqref{eq:strat_LP:cvx1} to \eqref{eq:strat_LP:cvx3} make sure that the result will be a convex combination of all the strategies, with the $\alpha$ variables being the coeficients of the convex combination.

Note that the realization probabilities may change when correcting other information sets. The bound from Theorem~\ref{lemma:alg-bound} on the error of a strategy constructed in this way however still holds. We have shown that the L1 distance of behavioral strategies $b^i$ in $I_1$ is at most $10^{-P}|\calA_1(I_1)|$ --- the distance to their convex combination $b$ cannot be larger.

We can use this LP to construct a valid strategy $\beta'_1$ from the result of the bilinear program in every imperfect recall information set where the results prescribe inconsistent behavior. We can use $\beta'_1$ to compute a lower bound $u_1(\beta'_1, \beta_2^{BR})$ where $\beta_2^{BR} \in BR(\beta'_1)$ on the overall expected maximin value of player 1. It is a valid lower bound, since this LP uses estimates on the expected loss and $\beta'_1$ has therefore no guarantees to be optimal.
